# Supplementary material for: DB-Nets: on The Marriage of Colored Petri Nets and Relational Databases
Source: arXiv:1611.03680 source file (2016-11-11)
Supplement: Supplementary file 1 [file appendix.tex]

\begin{example}\label{ex:oder-management}
The following persistence layer $\pers_{om} = \tup{\schema_{om},\cset_{om}}$ is designed to hold information that is used to model an order management scenario where a customer performs various activities while ordering products on an e-commerce website. In $\pers_{om}$'s typed database schema $\schema_{om}$ we reuse already defined data types $\typename{string}$ and $\typename{int}$, and introduce a new data type $\typename{status}$ specified as $\tup{\set{\cname{active},\cname{closed},\cname{rejected},\cname{accepted}},\set{=_{stat}}}$, where the comparison operator $=_{stat}$ functions exactly like  $=_s$. These types are used to define the following database relations:
\begin{compactitem}[$\bullet$]
\item $\relname{Product}(\typename{int},\typename{string})$ is a read-only binary relation containing information about products offered by the online store; $\relname{Product}(\cname{123},\cname{Nexus5})$  indicates that $\cname{Nexus5}$ with a warehouse product ID $\cname{123}$ is currently available on the website.
\item $\relname{Customer}(\typename{int},\typename{string})$ models customers currently registered on the store's website; for example, $\relname{Customer}(\cname{5},\cname{JohnDoe})$ means that a customer with a user name $\cname{JohnDoe}$ is registered to the system with a UID $\cname{5}$.
\item $\relname{Order}(\typename{int},\typename{int},\typename{status})$ is a trenary relation that represents all customer's orders together with their statuses; $\relname{Order}(\cname{20},\cname{5},\cname{active})$ indicates a $\cname{JohnDoe}$'s currently $\cname{active}$ (i.e., it can be either canceled or purchased) order with an ID $\cname{20}$. 
\item $\relname{InOrder}(\typename{int},\typename{int})$ shows which products are currently present in which orders; for example, $\relname{InOrder}(\cname{123},\cname{20})$ means that a $\cname{Nexus5}$ (product ID $\cname{123}$) is now in the order $\cname{20}$. 
\item $\relname{DeliveryAddress}(\typename{int},\typename{string})$ represents an address to which all items listed in an order should be delivered.
\end{compactitem}
The persistence layer is also equipped with a set of various constraints over $\schema_{om}$ that can be divided in two groups: \emph{primary keys} (for example, $\forall pid,d,d'.\relname{Product}(pid,d)\wedge\relname{Product}(pid,d')\rightarrow d=d'$ means that the first element of the $\relname{Product}$ relation is its primary key) and \emph{foreign keys} (for example, $\forall pid,oid.\relname{InOrder}(pid,oid)\rightarrow\exists d.\relname{Product}(pid,d)$ shows that product IDs in $\relname{InOrder}$ should reference corresponding IDs in $\relname{Product}$). A comprehensive overview of various relational dependencies and conventional methods used to model them can be found in \cite{AbHV95}.

To make this scenario operational, one should introduce a data logic over $\pers_{om}$. Here the data logic actions $\actions_{om}$ should support five main functionalities: registration of a new customer, creation of a new order, order manipulation by means of adding and deleting items, and preparation of an order for warehouse checks and its further dispatch. 

The registration of a new customer is managed by an action $\actname{register}$ that, given a new customer ID and her name in its parameters $\apar{\actname{register}}=\tup{\pname{newCID,name}}$\footnote{For the simplicity of the notation we consider action names to be the actual action identifiers.}, adds to the underlying database a new $\relname{Customer}$ entry $\aadd{\actname{register}}=\set{\relname{Customer}(\pname{newCID,name})}$.
As soon as the customer is logged in, the online shop offers  a big variety of products to buy. In the back-end, the website creates a new order for the customer that can be later on used to add selected items. This is done with the help of an action that uses a new order ID and a customer ID from $\apar{\actname{createOrder}}=\tup{\pname{newOID}, \pname{CID}}$  to create a new $\cname{active}$ order $\aadd{\actname{createOrder}}=\set{\relname{Order}(\pname{newOID},\pname{CID},\cname{active})}$. 
Once made a choice, the customer can add a selected item to her order by calling an action $\actname{addItem}$ that adds a product with a $\pname{PID}$ identifier to the order $\pname{OID}$ by creating a new $\relname{InOrder}$ tuple using $\aadd{\actname{addItem}}=\set{\relname{InOrder}(\pname{PID},\pname{OID})}$. In turn, every item that has been added can be eventually deleted. To support this scenario we provide an action $\actname{removeItem}$ that takes $\apar{\actname{removeItem}}=\tup{\pname{PID}, \pname{OID}}$ as input and deletes an $\relname{InOrder}$ entry specified in $\adel{\actname{removeItem}}=\set{\relname{InOrder}(\pname{PID}, \pname{OID})}$.

To proceed with purchasing selected items, in the first place, the customer has to change her order status from $\cname{active}$ to $\cname{closed}$ using an action $\actname{closeOrder}$ with $\apar{\actname{closeOrder}}=\tup{\pname{OID}, \pname{CID}}$. To update the order status, $\add~\set{\relname{Order}(OID,CID,\cname{closed})}~\del~\set{\relname{Order}(OID,CID,\cname{active})}$. In fact, $\actname{closeOrder}$ is meant to perform a readoing nothing but performing an update over an order with an identifier $OID$. The closed order is then processed by the warehouse customer management system so to check the actual availability of the purchasing items. To represent this activity, we introduce an action $\actname{doWarehouseCheck}(OID, CID, status):\add~\set{\relname{Order}(OID,CID,status)}~\del~\set{\relname{Order}(OID,CID,\cname{closed})}$ using which a warehouse manager can assign a new $status$ (can be either $\cname{rejected}$ or $\cname{accepted}$) to a selected order. An accepted order is eventually dispatched to an $address$ provided by the customer using an action $\actname{askAddress}(OID,address): \add~\set{\relname{DeliveryAddress}(OID,address)}$.

In this example we do not provide any queries for the data logic layer. It is done due to their user-oriented origins: queries are used to support user needs in processing and retrieving information existing in the database and can be clearly defined only when having an entire application design specified. This observation gives us conceptual motivation to provide a missing ``link'' in the chain of the data-aware process modeling. 
\end{example}
